# Supplementary material for: ComDensE : Combined Dense Embedding of Relation-aware and Common Features for Knowledge Graph Completion
Source: arXiv:2206.14925 source file (2022-06-29)
Supplement: Supplementary file 1 [file supplementary.tex]

\clearpage

\begin{center}
    SUPPLEMENTARY MATERIAL
\end{center}
\subsection{Optimizing size of matrix}
In this table, we experiment 3 different sizes of matrices in design space of width 1 $\times$ CombinE, where we optimize the size of the matrix of CombinE.
\begin{table}[h]
\centering
\begin{tabular}{c|c|c}
\hline
\multicolumn{3}{c}{\textbf{size of matrix in CombinE (width 1 $\times$)}}\\
\hline
 & \textbf{FB15k-237} & \textbf{WN18RR}\\
 \hline
 \multicolumn{3}{c}{\textbf{256$\times d$}}\\
 \textbf{MRR} & .355 & .463 \\
 \textbf{HIT@10} & .534 & .526 \\
 \textbf{HIT@1} & .265 & .429\\
  \hline
 \multicolumn{3}{c}{\textbf{128$\times d$}}\\
 \textbf{MRR} & .352 & .451 \\
 \textbf{HIT@10} & .530 & .520 \\
 \textbf{HIT@1} & .263 & .410 \\
\hline
\end{tabular}
%}

%\caption{Result of vector ($v_r \in \Re^{(d_e+d_r) \times 1}$) add operation different only $\Omega_r$ from DensE. (+,-) denote the performance difference with ConvE.}
\caption{where $d := d_e + d_r$, and we experiment 2 different sizes of matrices in width $1 \times$ CombinE. We use 256 $\times d$ for CombinE.}
\label{table11}
\end{table}

\subsection{Optimizing width of common layer}
We comprehensively search optimal width of common layer in proposed CombinE (256 $\times d$), where the wide dense matrix extracts diverse common features.
\begin{table}[h]
\centering
\begin{tabular}{c|c|c}
\hline
\multicolumn{3}{c}{\textbf{width of common layer}}\\
\hline
 & \textbf{FB15k-237} & \textbf{WN18RR}\\
 \hline
 \multicolumn{3}{c}{\textbf{Width $\times$ 1}}\\
 \textbf{MRR} & .355 & .461 \\
 \textbf{HIT@10} & .534 & .530 \\
 \textbf{HIT@1} & .265 & .434 \\
 \hline
  \multicolumn{3}{c}{\textbf{Width $\times$ 2}}\\
 \textbf{MRR} & \textbf{.356} & .465 \\
 \textbf{HIT@10} & \textbf{.536} & .534 \\
 \textbf{HIT@1} & \textbf{.265} & .431 \\
 \hline
  \multicolumn{3}{c}{\textbf{Width $\times$ 5}}\\
 \textbf{MRR} & .353 & .458 \\
 \textbf{HIT@10} & .533 & .521 \\
 \textbf{HIT@1} & .263 & .426 \\
\hline
  \multicolumn{3}{c}{\textbf{Width $\times$ 10}}\\
 \textbf{MRR} & .350 & .457 \\
 \textbf{HIT@10} & .531 & .521 \\
 \textbf{HIT@1} & .261 & .429 \\
\hline
  \multicolumn{3}{c}{\textbf{Width $\times$ 50}}\\
 \textbf{MRR} & .345 & .473 \\
 \textbf{HIT@10} & .525 & .536 \\
 \textbf{HIT@1} & .257 & .441 \\
\hline
 \multicolumn{3}{c}{\textbf{Width $\times$ 100}}\\
 \textbf{MRR} & .344 & \textbf{.473} \\
 \textbf{HIT@10} & .524 & \textbf{.538} \\
 \textbf{HIT@1} & .254 & \textbf{.440} \\
 \hline
 \multicolumn{3}{c}{\textbf{Width $\times$ 200}}\\
 \textbf{MRR} & .344 & .471 \\
 \textbf{HIT@10} & .524 & .541 \\
 \textbf{HIT@1} & .255 & .437 \\
\hline
\hline
\end{tabular}
%}

%\caption{Result of vector ($v_r \in \Re^{(d_e+d_r) \times 1}$) add operation different only $\Omega_r$ from DensE. (+,-) denote the performance difference with ConvE.}
\caption{Increasing width of common feature extraction layer and its performances on both FB15k-237 and WN18RR.}
\label{table12}
\end{table}

\newpage

\subsection{Optimizing both feature extraction layers}
We extensively experiment depth of both two feature extraction layers in CombinE, confirming whether increasing complexity of network has a positive effect or not.
\begin{table}[h]
\centering
\begin{tabular}{c|c|c}
\hline
\multicolumn{3}{c}{\textbf{depth of both common and relation-aware layer}}\\
\hline
 & \textbf{FB15k-237} & \textbf{WN18RR}\\
 \hline
  \multicolumn{3}{c}{\textbf{Depth-1}}\\
 \textbf{MRR} & \textbf{.356} & \textbf{.473} \\
 \textbf{HIT@10} & \textbf{.536} & \textbf{.538} \\
 \textbf{HIT@1} & \textbf{.265} & \textbf{.440} \\
 \hline
   \multicolumn{3}{c}{\textbf{Depth-2}}\\
 \textbf{MRR} & .338 & .454 \\
 \textbf{HIT@10} & .517 & .520 \\
 \textbf{HIT@1} & .248 & .419 \\
 \hline
   \multicolumn{3}{c}{\textbf{Depth-3}}\\
 \textbf{MRR} & .339 & .458 \\
 \textbf{HIT@10} & .513 & .524 \\
 \textbf{HIT@1} & .251 & .424 \\
\hline
\label{table12}
\end{tabular}
%}

%\caption{Result of vector ($v_r \in \Re^{(d_e+d_r) \times 1}$) add operation different only $\Omega_r$ from DensE. (+,-) denote the performance difference with ConvE.}
\caption{Increasing depth of both common and relation-aware feature extraction layer in CombinE and its performances on both FB15k-237 and WN18RR.}
\label{table13}
\end{table}
